# Supplementary material for: The Compositional Structure of Bayesian Inference
Source: arXiv:2305.06112 source file (2023-07-20)
Supplement: Supplementary file 1 [file binv-supp-lhs.tex]

% https://varkor.github.io/tangle/?t=W1tbXV0sW1tbMCxbXV0sWzAsW11dLFswLFtdXSxbMCxbXV0sWzAsW11dLFswLFtdXSxbMCxbXV0sWzAsW11dXSxbWzAsW11dLFswLFtdXSxbMCxbXV0sWzIsWzJdXSxbMSxbMCwxLDAsMV1dLFsxLFswLDEsMCwxXV0sWzEsWzAsMSwwLDFdXSxbMSxbMCwxLDAsMV1dXSxbWzEsWzAsMSwwLDBdXSxbMSxbMCwxLDAsMV1dLFsxLFswLDEsMCwxXV0sWzEsWzEsMCwxLDFdXSxbMCxbXV0sWzAsW11dLFswLFtdXSxbMCxbXV1dLFtbMCxbXV0sWzAsW11dLFswLFtdXSxbMixbMV1dLFsxLFswLDEsMCwxXV0sWzEsWzAsMSwwLDFdXSxbMSxbMCwxLDAsMV1dLFsxLFswLDEsMCwxXV1dLFtbMCxbXV0sWzAsW11dLFswLFtdXSxbMCxbXV0sWzAsW11dLFswLFtdXSxbMCxbXV0sWzAsW11dXV0sW1swLDQuNSwxLjUsWyIiXV0sWzAsNiwxLjUsWyJmX3AiLDEsMV1dLFswLDcuNSwxLjUsWyIiXV0sWzAsMiwyLjUsWyJmIiwxLDFdXSxbMCwwLjUsMi41LFsicCIsMCwxXV1dLFtbNywxLDAsIlgiXSxbNywzLDAsIlkiXV1d&c=F5A3A3,F5CCA3,F5F5A3,CCF5A3,A3F5A3,A3F5CC,A3F5F5,A3CCF5,A3A3F5,CCA3F5,F5A3F5,F5A3CC
\begin{tangle}{(8,5)}
	\tgBlank{(0,0)}{white}
	\tgBlank{(1,0)}{white}
	\tgBlank{(2,0)}{white}
	\tgBlank{(3,0)}{white}
	\tgBlank{(4,0)}{white}
	\tgBlank{(5,0)}{white}
	\tgBlank{(6,0)}{white}
	\tgBlank{(7,0)}{white}
	\tgBlank{(0,1)}{white}
	\tgBlank{(1,1)}{white}
	\tgBlank{(2,1)}{white}
	\tgBorderC{(3,1)}{1}{white}{white}
	\tgBorderA{(4,1)}{white}{white}{white}{white}
	\tgBorder{(4,1)}{0}{1}{0}{1}
	\tgBorderA{(5,1)}{white}{white}{white}{white}
	\tgBorder{(5,1)}{0}{1}{0}{1}
	\tgBorderA{(6,1)}{white}{white}{white}{white}
	\tgBorder{(6,1)}{0}{1}{0}{1}
	\tgBorderA{(7,1)}{white}{white}{white}{white}
	\tgBorder{(7,1)}{0}{1}{0}{1}
	\tgBorderA{(0,2)}{white}{white}{white}{white}
	\tgBorder{(0,2)}{0}{1}{0}{0}
	\tgBorderA{(1,2)}{white}{white}{white}{white}
	\tgBorder{(1,2)}{0}{1}{0}{1}
	\tgBorderA{(2,2)}{white}{white}{white}{white}
	\tgBorder{(2,2)}{0}{1}{0}{1}
	\tgBorderA{(3,2)}{white}{white}{white}{white}
	\tgBorder{(3,2)}{1}{0}{1}{1}
	\tgBlank{(4,2)}{white}
	\tgBlank{(5,2)}{white}
	\tgBlank{(6,2)}{white}
	\tgBlank{(7,2)}{white}
	\tgBlank{(0,3)}{white}
	\tgBlank{(1,3)}{white}
	\tgBlank{(2,3)}{white}
	\tgBorderC{(3,3)}{0}{white}{white}
	\tgBorderA{(4,3)}{white}{white}{white}{white}
	\tgBorder{(4,3)}{0}{1}{0}{1}
	\tgBorderA{(5,3)}{white}{white}{white}{white}
	\tgBorder{(5,3)}{0}{1}{0}{1}
	\tgBorderA{(6,3)}{white}{white}{white}{white}
	\tgBorder{(6,3)}{0}{1}{0}{1}
	\tgBorderA{(7,3)}{white}{white}{white}{white}
	\tgBorder{(7,3)}{0}{1}{0}{1}
	\tgBlank{(0,4)}{white}
	\tgBlank{(1,4)}{white}
	\tgBlank{(2,4)}{white}
	\tgBlank{(3,4)}{white}
	\tgBlank{(4,4)}{white}
	\tgBlank{(5,4)}{white}
	\tgBlank{(6,4)}{white}
	\tgBlank{(7,4)}{white}
	\tgRestr{(4,1)}{}
	\tgCell[(1,1)]{(5.5,1)}{f_p^\sharp}
	\tgIncl{(7,1)}{}
	\tgCell[(1,1)]{(1.5,2)}{f}
	\tgCell[(0,1)]{(0,2)}{p}
	\tgAxisLabel{(8,1.5)}{west}{X}
	\tgAxisLabel{(8,3.5)}{west}{Y}
\end{tangle}
