# Supplementary material for: The Compositional Structure of Bayesian Inference
Source: arXiv:2305.06112 source file (2023-07-20)
Supplement: Supplementary file 5 [file kernel-supp-restriction-lhs.tex]

% https://varkor.github.io/tangle/?t=W1tbXV0sW1tbMCxbXV0sWzAsW11dXSxbWzEsWzAsMSwwLDFdXSxbMSxbMCwxLDAsMV1dXSxbWzAsW11dLFswLFtdXV1dLFtbMCwxLDEuNSxbImZfcCIsMSwxXV1dLFtbMCwxLDIsIlhfcCJdLFsxLDEsMCwiWV97ZnB9Il1dXQ==&c=F5A3A3,F5CCA3,F5F5A3,CCF5A3,A3F5A3,A3F5CC,A3F5F5,A3CCF5,A3A3F5,CCA3F5,F5A3F5,F5A3CC
\begin{tangle}{(2,3)}
	\tgBlank{(0,0)}{white}
	\tgBlank{(1,0)}{white}
	\tgBorderA{(0,1)}{white}{white}{white}{white}
	\tgBorder{(0,1)}{0}{1}{0}{1}
	\tgBorderA{(1,1)}{white}{white}{white}{white}
	\tgBorder{(1,1)}{0}{1}{0}{1}
	\tgBlank{(0,2)}{white}
	\tgBlank{(1,2)}{white}
	\tgCell[(1,1)]{(0.5,1)}{\restr f p}
	\tgAxisLabel{(0,1.5)}{east}{X_p}
	\tgAxisLabel{(2,1.5)}{west}{Y_{f \circ p}}
\end{tangle}
