# Supplementary material for: The Compositional Structure of Bayesian Inference
Source: arXiv:2305.06112 source file (2023-07-20)
Supplement: Supplementary file 9 [file supp-object-strict-eq-lhs.tex]

% https://varkor.github.io/tangle/?t=W1tbXV0sW1tbMCxbXV0sWzAsW11dLFswLFtdXSxbMCxbXV1dLFtbMSxbMCwxLDAsMV1dLFsxLFswLDEsMCwxXV0sWzEsWzAsMSwwLDFdXSxbMSxbMCwxLDAsMV1dXSxbWzAsW11dLFswLFtdXSxbMCxbXV0sWzAsW11dXV0sW1swLDEsMS41LFsiIl1dLFswLDIuNSwxLjUsWyJmIiwxLDFdXV0sW1swLDEsMiwiWF9wIl0sWzMsMSwwLCJZIl1dXQ==&c=F5A3A3,F5CCA3,F5F5A3,CCF5A3,A3F5A3,A3F5CC,A3F5F5,A3CCF5,A3A3F5,CCA3F5,F5A3F5,F5A3CC
\begin{tangle}{(4,3)}
	\tgBlank{(0,0)}{white}
	\tgBlank{(1,0)}{white}
	\tgBlank{(2,0)}{white}
	\tgBlank{(3,0)}{white}
	\tgBorderA{(0,1)}{white}{white}{white}{white}
	\tgBorder{(0,1)}{0}{1}{0}{1}
	\tgBorderA{(1,1)}{white}{white}{white}{white}
	\tgBorder{(1,1)}{0}{1}{0}{1}
	\tgBorderA{(2,1)}{white}{white}{white}{white}
	\tgBorder{(2,1)}{0}{1}{0}{1}
	\tgBorderA{(3,1)}{white}{white}{white}{white}
	\tgBorder{(3,1)}{0}{1}{0}{1}
	\tgBlank{(0,2)}{white}
	\tgBlank{(1,2)}{white}
	\tgBlank{(2,2)}{white}
	\tgBlank{(3,2)}{white}
	\tgIncl{(0.5,1)}{}
	\tgCell[(1,1)]{(2,1)}{f}
	\tgAxisLabel{(0,1.5)}{east}{X_p}
	\tgAxisLabel{(4,1.5)}{west}{Y}
\end{tangle}
